# Supplementary material for: TextCraftor: Your Text Encoder Can be Image Quality Controller
Source: arXiv:2403.18978 source file (2024-03-27)
Supplement: Supplementary file 1 [file 6_supp.tex]

\textcolor{blue}{We include additional ablation studies and discussions in the Appendix: 
Denoising scheduler and steps. 
Weights of different reward functions. 
Analysis of Training Cost and the Amount of Training Data.
}

\subsection{Prompt Embedding Interpretability}
\textcolor{blue}{checking with Xian, maybe in appendix.}
